# Supplementary material for: Answering Counting Queries over DL-Lite Ontologies
Source: arXiv:2009.09801 source file (2020-09-02)
Supplement: Supplementary file 1 [file 9-appendix.tex]

% Appendix

\section{Proofs from Section}

%See Appendix \ref{appendex}.

\begin{proof}[Proof of Lemma \ref{interleavingismodel}]
Left to the reader ?
\end{proof}

\begin{proof}[Proof of Lemma \ref{rho}]
We prove that $\rho$ is well-defined, that is, $\rho(f'(d))$ does not depend on the choice of $d$. Assume we have $d_1$, $d_2$ such that $f'(d_1) = f'(d_2)$.

Since $f'$ maps to $\domain{*} \sqcup \domain{Can(\kb)}$, we have two cases to take care of :

\begin{itemize}

\item
if $f'(d_1), f'(d_2) \in \domain{*}$, that means $f'(d_1) = f(d_1)$ and $f'(d_2) = f(d_2)$, thus ensuring $f(d_1) = f(d_2)$.

\item
if $f'(d_1), f'(d_2) \in \domain{Can(\kb)}$, that means $f'(d_1) = d_1$ and $f'(d_2) = d_2$, thus ensuring again $f(d_1) = f(d_2)$.

\end{itemize}

One can conclude the proof by checking $\rho$ is indeed a homomorphism.
\end{proof}

Properties of the equivalence relations... 

\begin{lemma}
\label{funlem}

Assume you have $d, d' \in \domain{\I'}$, such that $(d, d') \in R^{\I'}$. For any $e \in \domain{\I'}$, we have :

If $e \sim d$, there exists $e' \in \domain{\I'}$ such that :
\begin{itemize}
\item  $(e, e') \in R^{\I'}$
\item  $e' \sim d'$.
\end{itemize}

Furthermore, if $e \notin \domain{*}$, such an element $e'$ is unique.

\end{lemma}

\begin{proof}

If $e \in \domain{*}$, then $d = e$, and $e' := d'$ obviously works.

Else, if $d, e \in \domain{\I'} \setminus \domain{*}$.

If $d' \in \domain{*}$, then we must define $e' := d'$, which is the unique way to satisfy $e' \sim d'$. Furthermore, since $(d, d') \in R^{\I'}$, it means we have $(d, \delta') \in R^{Can(\kb)}$, with $f'(\delta') = d'$.

Since $d \notin \individuals$ and $d, \delta' \in \domain{Can(\kb)}$, we know that either $\delta' = d S$ or $d = \delta' S^- $ for some role $S$ such that $\kb \models S \sqsubseteq R$. In the first case, since $d \sim e$, we have $\chi_e(\omega^0_e S) = \chi_d(\omega^0_d S) = d'$, thus the element $\epsilon' := r_e \omega^0_e S$ is so that $(e, \epsilon') \in R^{Can(\kb)}$ and $f'(\epsilon') = e'$, ensuring that $(e, e') \in R^{\I'}$. The second case is similar, but with $\epsilon'$ being the concatenation of $r_e$ and $\omega_e^0$ in which we drop the last letter $S^-$, since we know $\omega_e^0$ ends with $S^-$.

Otherwise, we also have $d' \in \domain{\I'} \setminus \domain{*}$. Thus, either $d' = d S$ or $d = d' S^-$, for some role $S$ such that $\kb \models S \sqsubseteq R$. Since we know the length of both $d$ and $d'$ modulo $k \geq 2$, those two cases are mutually exclusive (which is important for unicity). And we can build $e' := e S$ in the first case, and $e =: e' S^-$ in the second case.

\end{proof}

\begin{lemma}
\label{funlemgen}

Now, assume we have an element $e_1$, and for each $i$, two elements $d_i$, $d'_i$ such that : $d'_1 \sim e_1$ and  $d_i \sim d_i'$ and $(d_{i-1}, d_i) \in R^{\I'}_i, (d_i', d'_{i+1}) \in R_{i+1}^{\I'}$.

Applying Lemma \ref{funlem} $l-1$ times provide elements $e_2$, $e_3$, ... $e_l$ such that $e_1 \sim d_i$ and $(e_i, e_{i+1}) \in R^{\I'}_i$ for each $i$.

\end{lemma}

\begin{remark}

Assume none of the $d_i$ nor the $d'_i$ are in $\domain{*}$, and that we know some $d''_1$ and $d''_l$ such that $d_1'' \sim d_1$ and $d''_l \sim d_l$ and $(d_1'', d_l'') \in R^{\I'}$ for some role $R$, then, the uniqueness ensured at each step guarantees that $(e_1, e_l) \in R^{\I'}$.

Inded, since $(d_l'', d_1'') \in (R^-)^{\I'}$ and $e_l \sim d_l''$, we have an unique $e_{l+1}$ such that $e_{l+1} \sim e_1$ and $(e_l, e_{l+1}) \in R^{\I'}$. Since $e_{l+1} \sim e_1$, if we take $k > l$, then their roots have the exact same length. But since there exists a path of length $l+1$ from $e_1$ to $e_{l+1}$, their roots must be equal. Since they have same path from their root to themselves, they are equal, that is $e_1 = e_{l+1}$.

\end{remark}
